# Supplementary material for: PEFT-as-an-Attack! Jailbreaking Language Models during Federated Parameter-Efficient Fine-Tuning
Source: arXiv:2411.19335 source file (2024-12-19)
Supplement: Supplementary file 1 [file appendix.tex]

\subsection{Additional Experimental Results}

Figure~\ref{atk_local_20} shows the results of aggregation rules using 20 steps of local updates, i.e., $E_l=20$. The observed robustness patterns are partially consistent with those described Section~\ref{sec_agg} where we set $E_l=1$, i.e., traditional GARs (i.e., \median~\cite{yin2018byzantine}, \tm~\cite{yin2018byzantine}, and \gm~\cite{pillutla2022robust}) still exhibit greater vulnerabilities to attacks compared to EGARs. However, Figure~\ref{atk_local_20} reveals a greater diversity in the robustness of aggregation rules when utilizing the Fashion MNIST dataset. Particularly, the SignFlipping attack causes a significant accuracy drop to most defenses when down to $15\%$ of the clients are malicious. Notably, \clippedclustering exhibits effective defense against all examined attacks without substantial degradation in performance, whereas other aggregation rules manifest vulnerabilities to specific attack types.

\begin{figure*}[ht]
	\begin{subfigure}[b]{\linewidth}
		\centering
		\includegraphics[width=\linewidth]{./figs/fashion_mnist_local_20}
	\end{subfigure}
	\begin{subfigure}[b]{\linewidth}
		\centering
		\includegraphics[width=\linewidth]{./figs/cifar10_local_20}
	\end{subfigure}
	\caption{Comparing state-of-the-art aggregation rules under various attacks on Fashion MNIST and CIFAR10 datasets with IID partition. Unlike the settings described in Section~\ref{sec_agg}, we utilize 20 steps for local updates (i.e., $E_l=20$). Similarly, traditional GARs (i.e., \median~\cite{yin2018byzantine}, \tm~\cite{yin2018byzantine}, and \gm~\cite{pillutla2022robust}) still exhibit greater vulnerabilities to attacks, whereas advanced EGARs display greater resilience against the majority of attacks. Notably, \clippedclustering exhibits effective defense against all examined attacks without substantial degradation in performance, whereas other aggregation rules manifest vulnerabilities to specific attack types.}
	\label{atk_local_20}
\end{figure*}
