# Supplementary material for: PEFT-as-an-Attack! Jailbreaking Language Models during Federated Parameter-Efficient Fine-Tuning
Source: arXiv:2411.19335 source file (2024-12-19)
Supplement: Supplementary file 2 [file section_appendix_template.tex]

\section{Fine-Tuning Templates}

We follow to use the Alpaca prompt template in the following for constructing supervised datasets for fine-tuning.

\label{sec_ft_template}
\begin{template}{Prompt Template}{trainprompt}\small
\textit{Below is an instruction that describes a task for the given context.
Write a response that appropriately completes the request.
\\
\#\#\#
Context: \{\textcolor{blue}{context}\} \\
\#\#\#
Instruction: \{\textcolor{blue}{instruction}\} \\
\#\#\# Response: \{\textcolor{blue}{response}\} }
\end{template}

\begin{template}{MetaMathQA Template}{trainprompt}\small
\textit{Below is an instruction that describes a task.
Write a response that appropriately completes the request.\textbackslash n\textbackslash n\#\#\#
Instruction:\textbackslash n\{instruction\}\textbackslash n\textbackslash n\#\#\# Response:}
\end{template}

\begin{template}{MedQA Template}{trainprompt}\small
\textit{\textcolor{blue}{Context}: As an experienced physician, please provide a concise yet thorough analysis of the following medical question. Limit your response to 400 words and ensure it ends with "The correct answer is: [your\_answer]". \\  \\
\textcolor{blue}{Instruction}:  \{input[`sent1']\} \\
Options: \\
A: \{input[`options\_0]\}; \\ 
B: \{input[`options\_1]\};  \\ 
C: \{input[`options\_2]\};  \\ 
D: \{input[`options\_3]\};\\ \\
Please analyze the question following these steps, being concise but comprehensive: \\ \\
1. Key Information Analysis: \\
  - Extract and list relevant patient details, symptoms, signs, and test results \\
  - Highlight only the most significant findings \\ 
2. Diagnostic Reasoning: \\
  - Identify the most likely diagnosis/clinical scenario \\
  - Note the key diagnostic indicators \\ \\
3. Option Analysis: \\
  - Explain why your answer is correct \\
  - Briefly state why other options are incorrect \\
4. Quick Summary: \\
  - List 2-3 key points that lead to the correct answer \\
  \\
Again, your analysis must: \\
- Be under 400 words \\
- Use clear, professional language \\
- Stay focused on key points \\
- End with exactly "The correct answer is: [your\_answer] \\
- You must make a choice among the options provided, even without complete confidence. \\
\\
Now begin your analysis.}
\end{template}
